# Supplementary material for: Prediction of Overall Survival of Brain Tumor Patients
Source: arXiv:1909.04596 source file (2019-09-10)
Supplement: Supplementary file 1 [file additional.tex]

\iffalse
% %------------Table 1-------------------- % %
\begin{table}[htbp]
	\caption{Features for SVM training.}
	\begin{center}
		\begin{tabular}{|c|c|}
			\hline
			\multicolumn{1}{|c|}{\textbf{Feature}} & \multicolumn{1}{c|}{\textbf{Detail}} \\ 
			\hline
			Age & \begin{tabular}[c]{@{}l@{}}Age of patient taken directly from \\ the BRATS 2017 dataset\end{tabular} \\ \hline
			Amount of Necrotic & \begin{tabular}[c]{@{}l@{}}\# of necrotic pixels / \# of total tumor \\ pixels\end{tabular} \\ \hline
			Amount of Edema & \begin{tabular}[c]{@{}l@{}}\# of edema pixels / \# of total tumor \\ pixels\end{tabular} \\ \hline
			Amount of Enhancing tumor & \begin{tabular}[c]{@{}l@{}}\# of enhancing tumor pixels / \# of total \\ tumor pixels\end{tabular} \\ \hline
			Amount of Tumor & \# of tumor pixels/ \# of brain pixels \\ \hline
		\end{tabular}
		\label{feature-table}
	\end{center}
\end{table}
\fi

% %------------Fig 3-------------------- % %
\begin{figure}[!h]
\centering

\subfloat[\label{fig}]{%
   \includegraphics[width=0.20\textwidth]{Brats17_CBICA_AOO_1_98.png}
 }
  \hfill
\subfloat[\label{fig2}]{%
   \includegraphics[width=0.20\textwidth]{Brats17_CBICA_AOO_1_98L.jpg}
 }
  \vfill
\subfloat[\label{fig3}]{%
   \includegraphics[width=0.20\textwidth]{Brats17_TCIA_199_1_82.png}
 }
  \hfill
\subfloat[\label{fig4}]{%
   \includegraphics[width=0.20\textwidth]{Brats17_TCIA_199_1_82L.jpg}
 }
 
 \caption{Segmentation results: a) Patient-1 segmented result, b) Patient-1 Ground Truth, c) Patient-2 segmented result, and d) Patient-2 Ground Truth. }
\label{CNN-Res}
\end{figure}
